# Supplementary material for: LongBoX: Evaluating Transformers on Long-Sequence Clinical Tasks
Source: arXiv:2311.09564 source file (2023-11-16)
Supplement: Supplementary file 1 [file 6_appendix.tex]

\section{Data Description}
\label{app:data_description}

In this section, we provide comprehensive information about each dataset, along with the diverse document types that were utilized for creating each dataset.

\subsection{Type of Data}
\paragraph{Discharge Summary} is a document containing details of why a person was admitted, diagnosis, medical regimen and response to it, medical condition at discharge time, and after discharge care such as medications to take at home \cite{kind2008documentation}. These summaries are in long text format but not organized. Further, datasets selected in \dataset{} used de-identified the summaries to respect the patient's privacy.

% \paragraph{Electronic Health Records}  is a complete record of a patient's medical history including diagnosis, treatments, medication, vitals, allergies, immunization, and laboratory tests. These records are lengthy and unstructured.

\paragraph{Progress Report} is a document that forms the basis of the next plan of treatment. It consists of assessment, diagnosis, planning, intervention, and evaluation.

\paragraph{Longitudinal Record} is a medical document that aggregates information from various sources in the health care system.

\subsection{Datasets}
\paragraph{Smoking 2006} dataset \cite{uzuner2008identifying} was released as part of the n2c2 challenge in 2006. Given the discharge summaries of patients, the task is to categorize the smoking status of a patient into: (1) Past Smoker, (2) Current Smoker, (3) Smoker, (4) Non-Smoker, and (5) Unknown. 

\paragraph{Obesity 2008} dataset \cite{uzuner2009recognizing} was collected for the n2c2 challenge in 2008. Based on discharge summaries, the task is to determine the presence of 15 different diseases such as asthma, depression, and diabetes. Any of these 15 diseases mentioned in the record then the patient is considered as obese. The aim here is to identify the presence of disease and categorize them into: (1) Present, (2) Absent, (3) Questionable, and (4) Unmentioned.

\paragraph{Assertions 2010} dataset \cite{uzuner20112010} is a part of the n2c2 challenge 2010. The data consists of discharge summaries as well as progress reports of patients. The task is to classify the occurrence of a concept into 6 categories which are "Present", "Absent", "Hypothetical", "Possible", "Associated with someone else" and "Conditional". The concept can be medical problems, treatments, and tests.

% \paragraph{N2C2 Relations challenge Relations} is an extension of assertions challenge. The dataset \cite{uzuner20112010} used is the same however here the task is to find the relation between two concepts. The relations are defined as - TrIP (treatment improves or cures the problem), TrWP (treatment worsens the problem), TrCP (treatment causes another medical problem), TrAP (treatment is given for a medical problem and outcome not mentioned), TrNAP (treatment was not given or discontinued owing to another medical problem not caused by the treatment),  TeRP (test reveals or indicates the medical condition), TeCP (test is conducted for diagnosing a medical problem and the outcome is not known), and PIP (medical problems that describe or reveal aspects of the same medical problem and those that cause other medical problem).

\paragraph{Temporal Relations 2012} dataset \cite{sun2013evaluating} released in 2012 n2c2 challenge. The dataset consists of discharge summaries. Given a clinically significant event and time entity, the task is to find the type of relationship between them - BEFORE (event happens before given temporal expression), AFTER (event happens after given temporal expression), SIMULTANEOUS (event happens on given temporal expression), OVERLAP (event overlaps with temporal expression), BEGUN\_BY (event started on given temporal expression), ENDED\_BY (event ended on given temporal expression), DURING (event happens during given temporal expression), and BEFORE\_OVERLAP (event started before and lasts during given temporal expression).

\paragraph{Heart Disease 2014} dataset \cite{kumar2015creation} released in 2014 n2c2 challenge and consists of longitudinal medical records. The task here is to find indicators of a given condition in the text and classify them into "Present" and "Not present". For instance, the indicator for Diabetes can be different aspects such as the patient mentioning having diabetes, high glucose, and high HBA1c levels.

\paragraph{Cohort Selection} dataset \cite{stubbs2019cohort} is released in the n2c2 challenge 2018. In this dataset, we classify whether the criteria are met or not met for clinical trials. Clinical trials have certain criteria for taking a patient into the trial groups. the dataset has defined 13 criteria such as MAJOR-DIABETES (Major diabetes-related complication), ALCOHOL-ABUSE (Current alcohol use over weekly recommended limits), and ENGLISH (Patient must speak English). 

% MAKES-DECISIONS (Patient must make their own medical decisions), ABDOMINAL (History of intraabdominal surgery, small or large intestine resection or small bowel obstruction),  MAJOR-DIABETES (Major diabetes-related complication), ADVANCED-CAD (Advanced cardiovascular disease), MI-6MOS (Myocardial infarction in the past 6 months), KETO-1YR (Diagnosis of ketoacidosis in the past year), DIETSUPP-2MOS (Taken a dietary supplement, excluding Vitamin D, in the past 2 months), ASP-FOR-MI (Use of aspirin to prevent myocardial infarction), HBA1C (HbA1c value between 6.5 and 9.5), CREATININE (Serum creatinine > upper limit of normal ).

\paragraph{ADE 2018} dataset \cite{henry20202018} was part of another n2c2 2018 challenge. Given discharge summaries, the task here is to classify the relationship between a drug and another related entity as Strength-Drug (e.g., 20mg), Dosage-Drug (e.g., 1 tab per day), Duration-Drug (e.g., 5-day course), Frequency-Drug (e.g., every 4-6 hrs), Form-Drug (e.g., tablet, capsule), Route-Drug (e.g., intraperitoneal, IM), Reason-Drug (reason/disease for which the medication is prescribed), and ADE-Drug (side effect caused by the drug).

% \paragraph{BioASQ8b} dataset is part of BIOASQ challenge. This is a QA dataset, given a context and question related to biology, the output should be an answer. Further, the questions in the data are phrased to get a summary based on the context of the question.  

% \begin{itemize}
%     \item Dataset task details (cite the papers for datasets)
%     \item Table for dataset statistics (total number of training samples, samples that exceed max\_length of LLMs, i.e., 1024 or 2048, or 4096)
% \end{itemize}
